# Supplementary material for: Electronic properties of substitutional impurities in graphene-like C$_2$N, $tg$-C$_3$N$_4$, and $hg$-C$_3$N$_4$
Source: arXiv:2010.09917 ancillary file (2020-10-19)
Supplement: Supplementary file 1 [file SM.pdf]

## Supplementary Materials (SM)

# Electronic properties of substitutional impurities in graphene-like $C_2N$, *tg*-$C_3N_4$, and *hg*-$C_3N_4$


Saif Ullah,[1]* Pablo A. Denis,[2] Marcos G. Menezes,[3†] Fernando Sato,[1] and Rodrigo B. Capaz[3]

1- Departamento de Física, Instituto de Ciências Exatas, Campus Universitário, Universidade Federal de Juiz de Fora, Juiz de Fora, MG 36036-900, Brazil

2- Computational Nanotechnology, DETEMA, Facultad de Química, UDELAR, CC 1157, 11800 Montevideo, Uruguay

3- Instituto de Física, Universidade Federal do Rio de Janeiro, Caixa Postal 68528, 21941-972, Rio de Janeiro, RJ, Brazil

*email:sullah@fisica.ufjf.br

†email:marcosgm@if.ufrj.br


**Notes**

In order to check the accuracy of our vdW-DF1 calculations, we further perform PBE-GGA calculations with PAW pseudopotentials as implemented in VASP code [1-5]. The kinetic energy cut off for the expansion of wavefunctions is set to 500 eV and the first Brillouin zone is sampled with a 3×3×1 K-point grid. A first order Methfessel-Paxton smearing method is employed in the calculations [6].

We begin by calculating the structural and electronic properties of pristine systems and by comparing them with our main results as well as with the reported literature. In table S1, we show the lattice constants, different C-C and C-N bond lengths, and electronic band gaps. As can be seen, there is an excellent agreement between our (PBE) results and that previously reported literature (with a PBE+D2 functional). Furthermore, these outcomes agree quite nicely with the vdW-DF1 results reported in the main text.

| **System** | **a (Ang)** | **$d_{C-C}$ (Ang)** | **$d_{C-N}$ (Ang)** | **$E_g$ (eV)** |
|---|---|---|---|---|
| | | **This Work** | | |
| **$C_2N$** | 8.332 | 1.43, 1.47 | 1.34(h) | 1.662 |
| ***tg*-$C_3N_4$** | 4.789 | | 1.33(h), 1.46 (l) | 1.576 |
| ***hg*-$C_3N_4$** | 7.1419 | | 1.33(h), 1.48(l), 1.39(c) | 1.2133 |

| Previous Work | | | | |
|---|---|---|---|---|
| **$C_2N$**[7] | 8.336 | 1.429, - | 1.336 | 1.66 |
| ***tg*-$C_3N_4$**[7] | 4.783 | | 1.326, 1.463 | 1.574 |
| ***hg*-$C_3N_4$**[7] | 7.134 | | 1.33, 1.475, 1.393 | 1.197 |

**Table S1:** *Comparison of structural and electronic properties of our PBE results with the previously reported PBE+D2.*

Next, we calculate and compare the energetics with different codes. To that end, we gathered in Table S2, the calculated formation and cohesive energies of the pristine and doped systems. As stated in the main text, the values of formation energy depend on its definition and the calculation method. For that reason, we provide for comparison, the formation energies calculated with a second definition:

$$E_f'[X(Y)] = E_t + \mu_Y - E_{pristine} - \mu_X,$$

where $E_t$ is the total energy of the system with the impurity and $E_{pristine}$ corresponds to the energy of the pristine material. Finally, $\mu_Y$ is the chemical potential of species $Y$, which is the dopant and $\mu_X$ is the chemical potential of the removed (replaced) atom.

As explained in the main text, the chemical potentials were taken from the most stable forms. The results are summarized in Table S2. Despite the numerical differences, we see an excellent agreement in the profile of formation energies calculated with different methods. Besides, both codes give similar qualitative results. In all the three structures, the find that the synthesis of B(C) is the easiest. For $C_2N$, we see that the integration of S(N) is favorable than N(C) and C(N), the latter being the least favorable. However, in *tg*-, and *hg*-$C_3N_4$, the second most favorable structure is found to be C(N). This can be attributed to the higher amount of N (than C) in these structures. Besides, the N(C) structure is found to be the least favorable in the latter two cases. Furthermore, for completeness, we also report the cohesive energies of every constituent used in the calculations. At vdW-DF1 level, the cohesive energy of B (alpha-sheet), C (graphene), N ($N_2$), and S (bulk) is -5.892, -7.516, -4.813, and -3.214 eV/atom, respectively. In the same manner, the cohesive energy at PBE-GGA level is -6.382, -7.934, -5.199, and -3.206 eV/atom, respectively.

We also calculate cohesive energy which provides an insight regarding the relative strength of these systems. Having said that, we find that the C(N) replacement is the most stable in all the structures—even stronger than the pristine systems—which can be attributed to the stronger C-C bonding. This behavior can also be understood from a comparison of the cohesive strength of the pure structures in which $C_2N$—where there are more C than N and the presence of C-C bonds—bears the strongest cohesive strength. In both the $C_3N_4$ structures, the B substitution is also more favorable than the undoped structures. This preference is a consequence of better B-N chemistry. Surprisingly, the S-doped systems have a better strength—despite its bigger size—than the N(C) systems. Consequently, an increase in C-C (or B-N) bondings adds to the stability, whereas, the opposite happens when we increase N-N bonds in the structures.

For comparison, we consider a 10 × 10 graphene supercell (for which the lattice constant is comparable to that of our 3 × 3 $C_2N$ supercell) doped with B, N, and S at vdW-DF1 level. The cohesive energy of pristine graphene is -7.516 eV/atom. With the introduction of these dopants, a slight increase in the cohesive energy is observed. The cohesive energies of B, N, and S doped graphene are -7.504, -7.498, and -7.474 eV/atom, respectively, in agreement with a previous report [8].

| **System** | **$E_f$ (eV/atom)** | | **$E'_f$ (eV)** | | **$E_c$ (eV/atom)** | |
|---|---|---|---|---|---|---|
| | **VASP** | **SIESTA** | **VASP** | **SIESTA** | **VASP** | **SIESTA** |
| **$C_2N$** | | | | | -6.7895 | -6.4088 |
| **B-C** | 0.2365 | 0.207470 | 0.5039 | 0.245199 | -6.7768 | -6.3973 |
| **C-N** | 0.2452 | 0.218200 | 1.9218 | 1.992500 | -6.7945 | -6.4132 |
| **N-C** | 0.2393 | 0.212687 | 0.9612 | 1.089280 | -6.7667 | -6.3854 |
| **S-N** | 0.2356 | 0.211000 | 0.357 | 0.826894 | -6.7750 | -6.3938 |
| ***tg*-$C_3N_4$** | | | | | -6.0303 | -5.6747 |
| **B-C** | 0.3303 | 0.283398 | -1.9494 | -2.334700 | -6.032 | -5.6788 |
| **C-N(h)** | 0.3504 | 0.306063 | 1.5686 | 1.631572 | -6.037 | -5.6808 |
| **C-N(l)** | | 0.300909 | | 0.729593 | | -5.6860 |
| **N-C** | 0.3619 | 0.316874 | 3.576 | 3.523450 | -5.994 | -5.6392 |
| **S-N(h)** | 0.3563 | 0.314078 | 2.596 | 3.034150 | -6.004 | -5.6483 |
| **S-N(l)** | | 0.324061 | | 4.781100 | | -5.6383 |
| ***hg*-$C_3N_4$** | | | | | -6.082 | -5.7108 |
| **B-C(l)** | 0.2739 | 0.242333 | -1.916 | -2.309945 | -6.085 | -5.7163 |
| **B-C(c)** | | 0.244323 | | -2.059262 | | -5.7143 |
| **C-N(c)** | | 0.266203 | | 0.697681 | | -5.7267 |
| **C-N(h)** | 0.3036 | 0.275590 | 1.8355 | 1.880400 | -6.0899 | -5.7173 |

| | | | | | | |
|---|---|---|---|---|---|---|
| **C-N(l)** | | 0.265217 | | 0.573413 | | -5.7277 |
| **N-C(l)** | 0.3154 | 0.286785 | 3.313 | 3.291020 | -6.034 | -5.6632 |
| **N-C(c)** | | 0.286111 | | 3.206109 | | -5.6639 |
| **S-N(c)** | | 0.311766 | | 6.438600 | | -5.6470 |
| **S-N(h)** | 0.2982 | 0.271987 | 1.1543 | 1.426381 | -6.057 | -5.6868 |
| **S-N(l)** | | 0.289412 | | 3.621990 | | -5.6694 |

**Table S2:** *A comparison of the $E_f$ (in eV/atom calculated with equation 2 in the main text), $E_f'$ (in eV calculated with the above equation) and Cohesive energy (in eV/atom) calculated at PBE-GGA (with the PW VASP code) and vdW-DF1 (with LCAO SIESTA code) level.*

In Table S3, we present the structural modifications induced due to the introduction of impurity atoms and the binding energies of the impurity levels, as given by the cross-check calculations. The results match quite well with the calculations performed with the SIESTA code, shown in Tables 3 and 4 of the main text.

| **System** | **$d_{1st}$ (Å)** | **$E_b$(eV)** |
|---|---|---|
| | **$C_2N$** | |
| **B-C** | 1.39 (B-N) 1.54, 1.57 (B-C) | 0.5158047, 0.0875 |
| **C-N** | 1.37 | 1.0273 |
| **N-C** | 1.38 (N-N) 1.41 (N-C) | 0.136401 |
| **S-N** | 1.73 | 0.469903 |
| | ***tg*-$C_3N_4$** | |
| **B-C** | 1.42 (h), 1.49 (l) | 0.1658002, 0.0369 |
| **C-N(h)** | 1.38 | 1.3850011 |
| **N-C** | 1.35 (h). 1.45 (l) | 0.71270129 |
| **S-N(h)** | 1.72 | 0.1385958 |
| | ***hg*-$C_3N_4$** | |
| **B-C(l)** | 1.42 (h), 1.51 (l) | 0.092404 |
| **C-N(h)** | 1.39 average | 1.0821828, 0.0834 |
| **N-C(l)** | 1.34 (h), 1.47 (l) | 1.0821828 |
| **S-N(h)** | 1.765 average | 0.09969952 |

**Table S3:** *Structural modifications caused by the impurity atoms along with the binding energies (in eV) as given by PBE-GGA calculations in VASP.*

Finally, we calculate the electronic properties of the pristine and doped systems at the PBE-GGA level as implemented in VASP. The electronic band structures for pristine systems (supercells) are given in Figure S1. In addition, due to the indirect gap nature in *hg*-$C_3N_4$, we also include the unit cell band structure for clarity. The electronic band structures are in excellent agreement with those shown in the main text and with earlier published data. Having said that, our vdW-DF1 calculations correctly captured the direct and indirect band gaps. The main difference lies in the magnitude of the band gaps, for which the vdW-DF1 values reported in the main text are consistently higher and more accurate than the PBE-GGA values reported here. In fact, the underestimation of band gaps in PBE is a known issue and comes from the semi-local nature of the exchange-correlation functional. The electronic band structures for the selected doped systems can be appreciated in Figures S2-S5, where a similar level of agreement is found with the results reported in the corresponding figures of the main text. A small disagreement, however, is found in the B(C) impurity in $C_2N$, where an additional impurity level appears inside the gap in the spin-polarized calculation (Fig. S3). Such a difference can be attributed to the underestimation of the band gap in PBE, as discussed in the caption of the Figure.

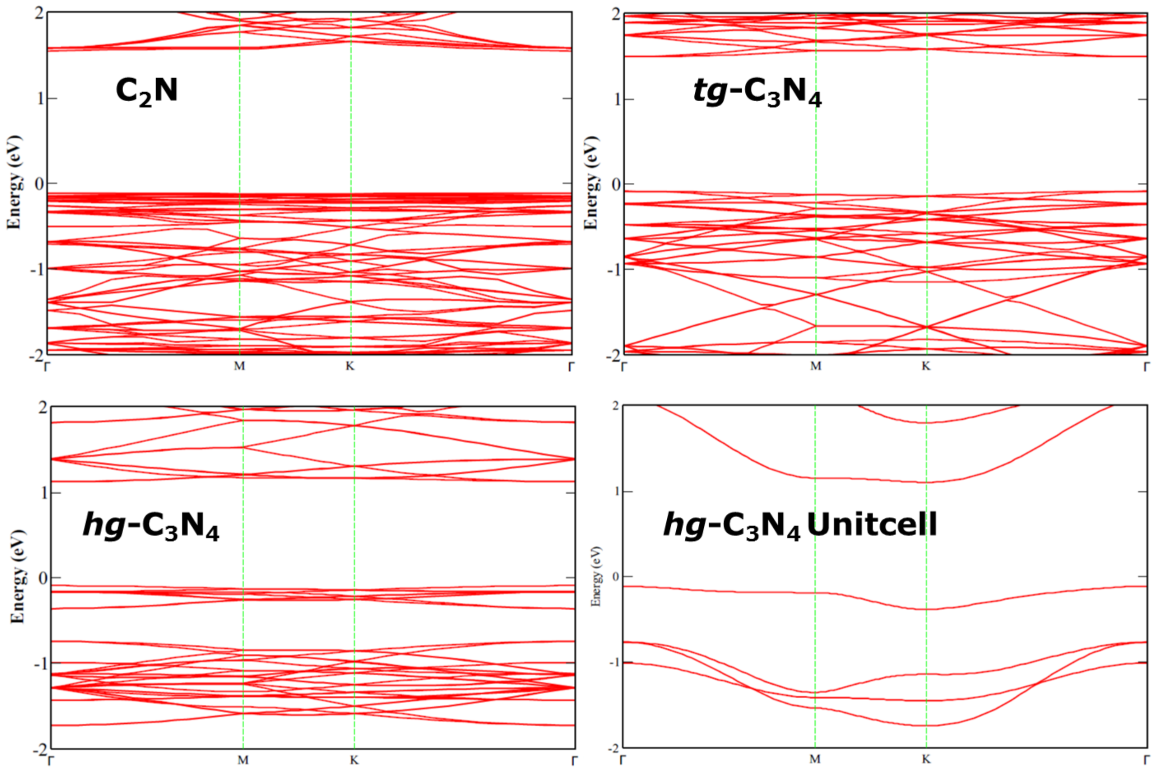

**Figure S1:** *Electronic band structures for the pristine systems (supercells), as given by the PBE-GGA calculation in VASP. For better visualization of the indirect gap nature of hg-$C_3N_4$, the unit cell band structure is also given.*

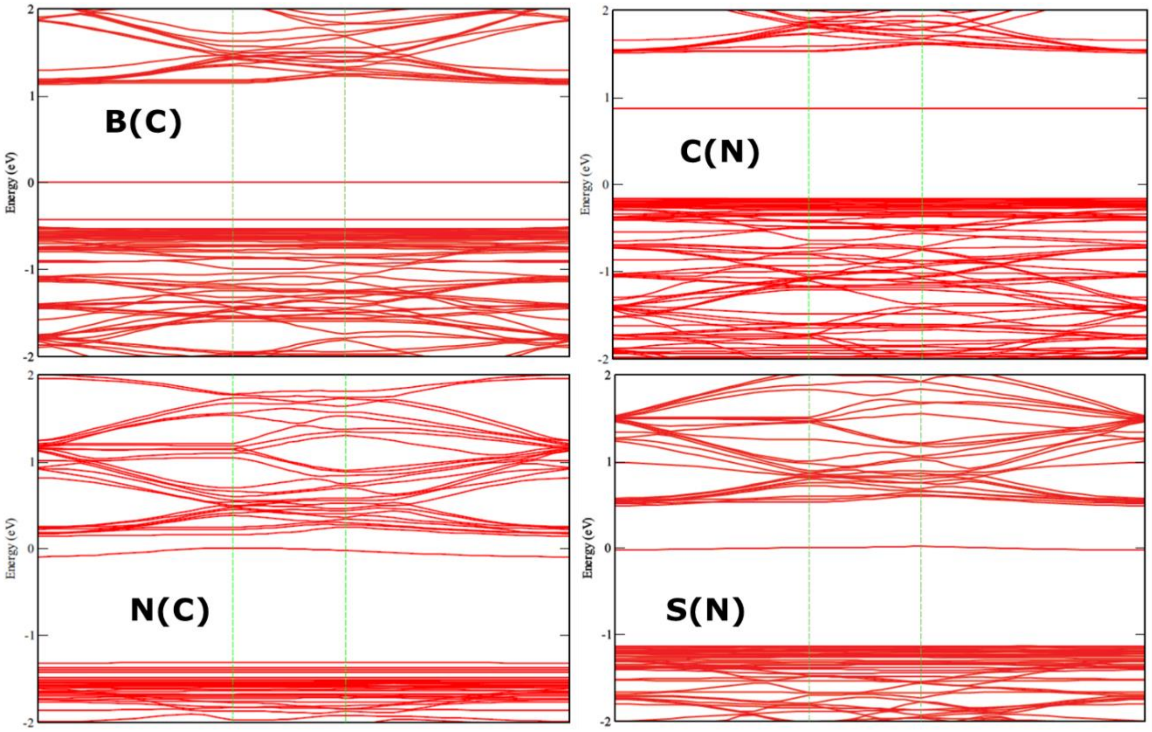


**Figure S2:** *Electronic band structures of doped $C_2N$ at the PBE-GGA level.*

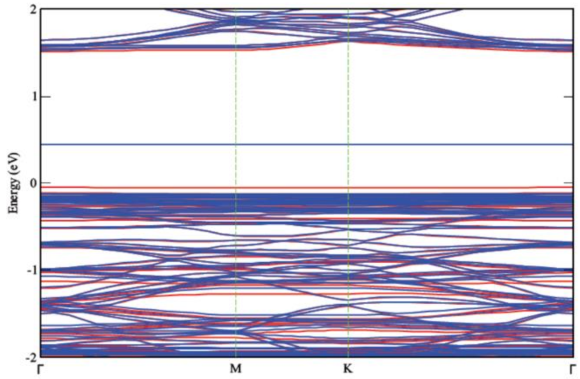


**Figure S3:** *Spin polarized electronic band structure of B(C) in $C_2N$ (at the PBE-GGA level). In this case, spin up (red) and down (blue) impurity levels are found inside the gap, in contrast with the vdW-DF1 result shown in Fig. 6 of the main text, where a single channel is found inside the gap. This is probably due to the underestimation of the gap in PBE, which results in a smaller spin*

splitting. For all the other dopants, the impurity level structures of PBE and vdW-DF1 are found to be the same.

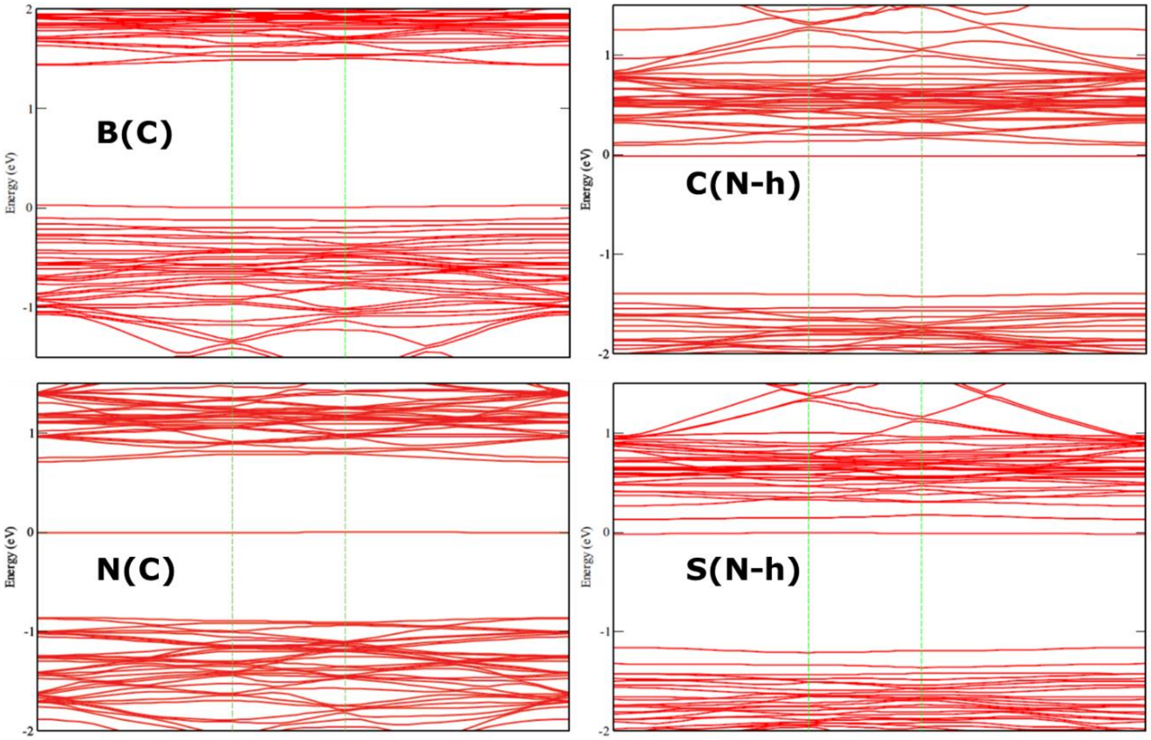


**Figure S4**: *Electronic band structures of doped tg-$C_3N_4$ at the PBE-GGA level.*

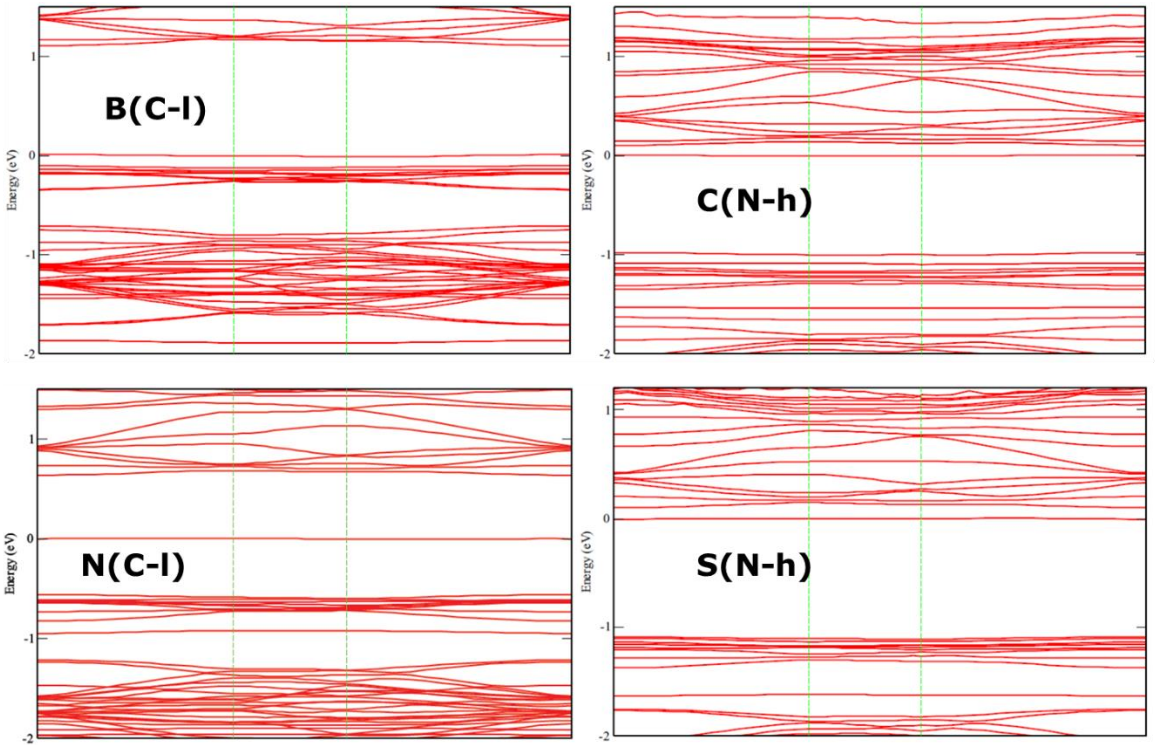


**Figure S5:** *Electronic band structure of doped hg-$C_3N_4$ at the PBE-GGA level.*

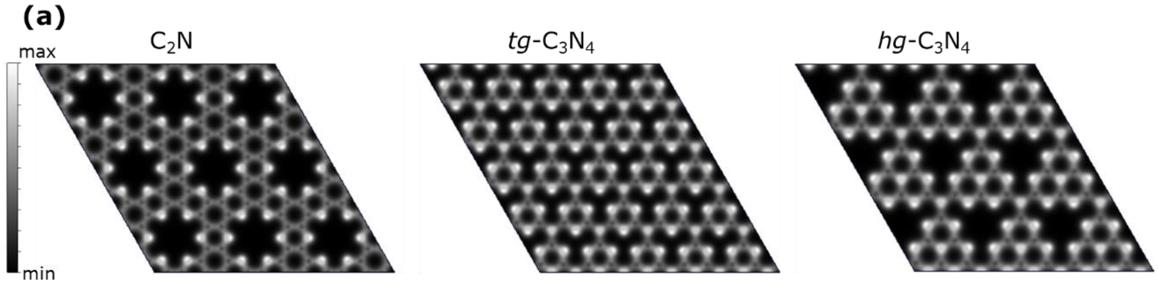

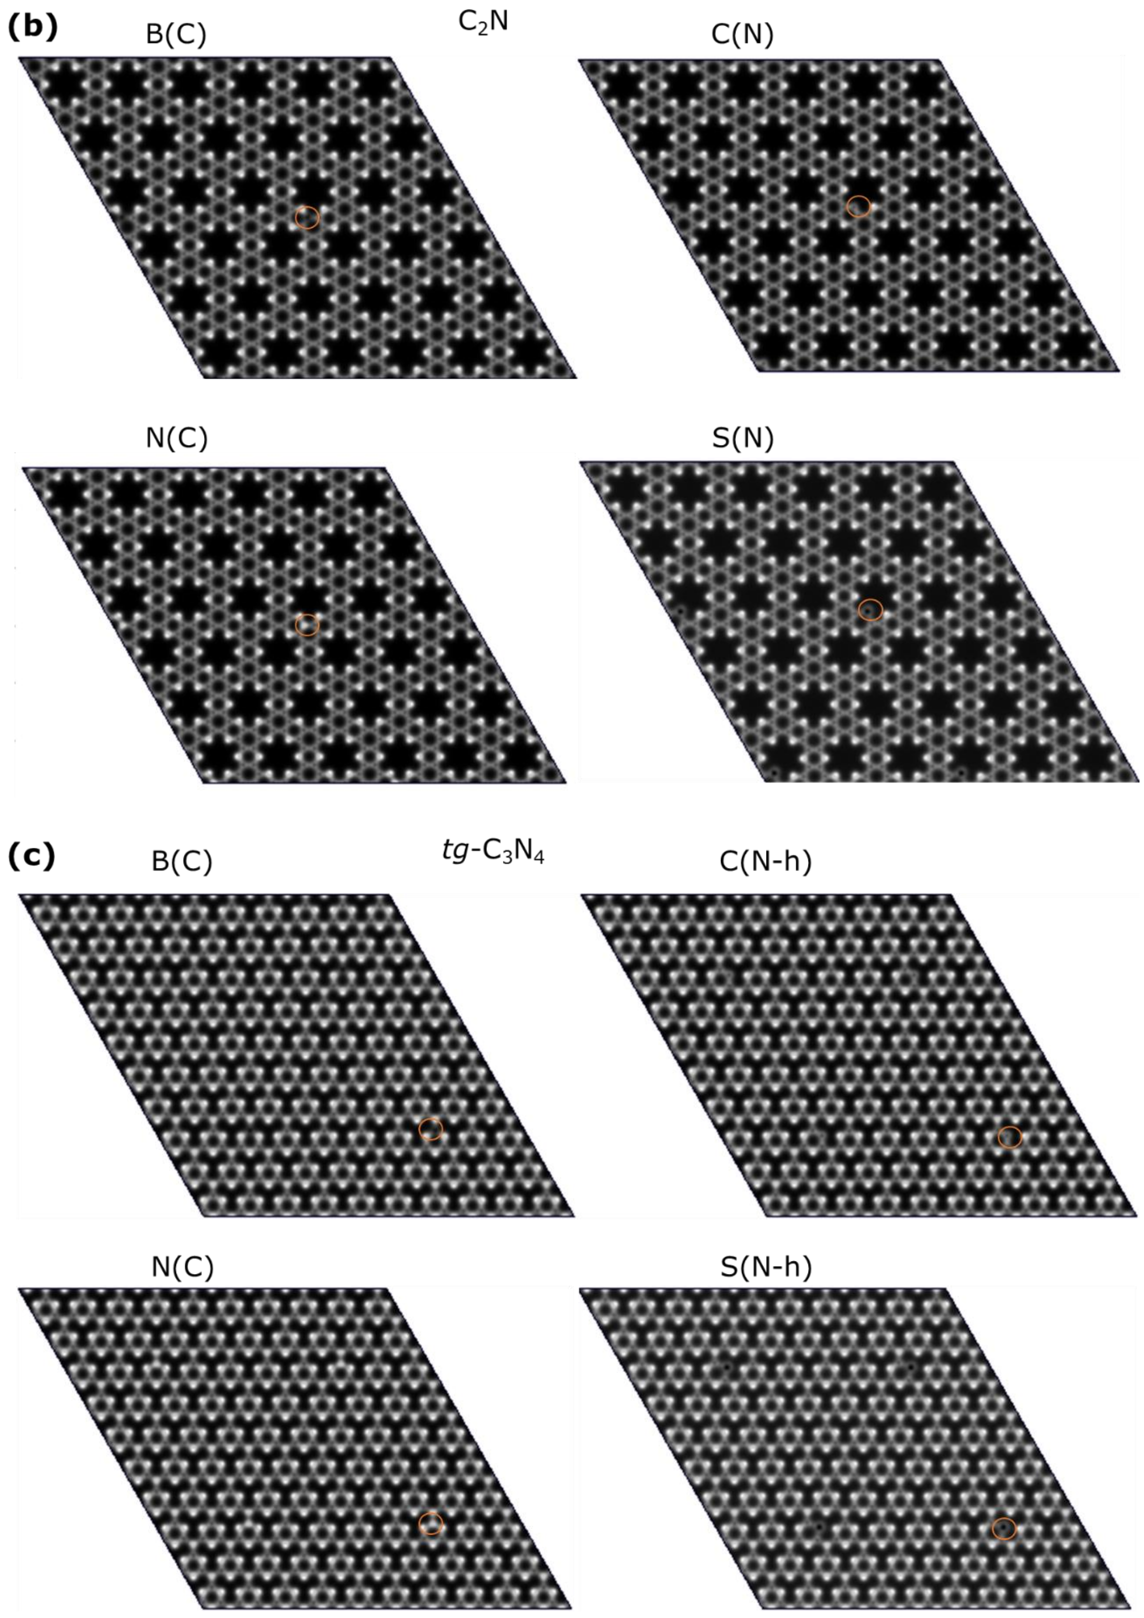
(b)
C2N
B(C)
C(N)
N(C)
S(N)
(c)
tg-C3N4
B(C)
C(N-h)
N(C)
S(N-h)

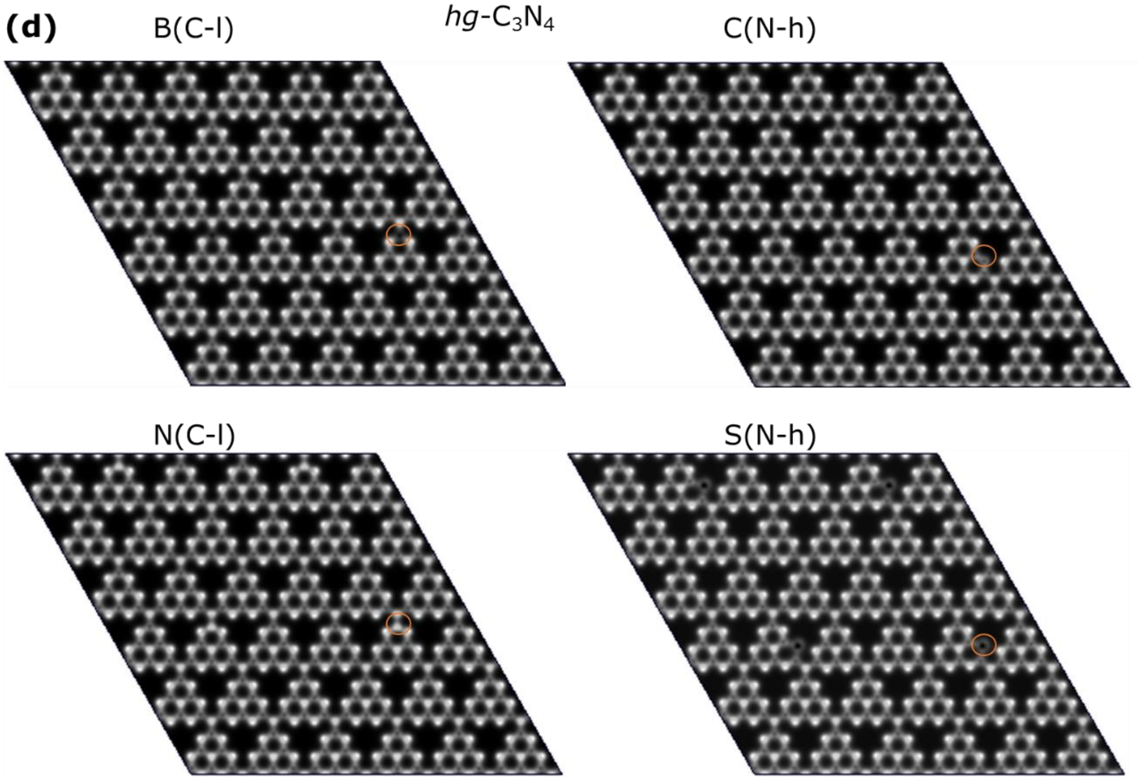


**Figure S6:** 2D cut of total density of states of (a) pristine structures, (b) doped $C_2N$, (c) doped *tg*-$C_3N_4$, and (d) doped *hg*-$C_3N_4$. In doped structures, the position of impurity is indicated by an orange line.

## References

1 G. Kresse and J. Hafner, Physical Review B **49**, 14251 (1994).
2 J. P. Perdew, K. Burke, and M. Ernzerhof, Physical review letters **77**, 3865 (1996).
3 J. P. Perdew, K. Burke, and M. Ernzerhof, Physical review letters **78**, 1396 (1997).
4 P. E. Blöchl, Physical Review B **50**, 17953 (1994).
5 G. Kresse and J. Furthmüller, Computational Materials Science **6**, 15 (1996).
6 M. Methfessel and A. T. Paxton, Physical Review B **40**, 3616 (1989).
7 M. Makaremi, S. Grixti, K. T. Butler, G. A. Ozin, and C. V. Singh, ACS Applied Materials & Interfaces **10**, 11143 (2018).
8 S. Ullah, P. A. Denis, and F. Sato, ChemPhysChem **18**, 1864 (2017).
